# Supplementary material for: Hearing-Loss Compensation Using Deep Neural Networks: A Framework and Results From a Listening Test
Source: arXiv:2403.10420 source file (2024-12-13)
Supplement: Supplementary file 1 [file appendix.tex]

\section{Appendix}
\subsection{Hearing loss compensation}

We construct a very simple model of the auditory system, using a gammetone filterbank. In frequency-space, define the normal hearing model and the hearing impaired model as respectively $\textbf{N} \in \mathbb{C}^{num_{CF}\times f_{bins}}$ and $\textbf{H}  \in \mathbb{C}^{num_{CF}\times f_{bins}}$, and a compensation-vector, i.e. a compensation strategy applied to the hearing-impaired model at each frequency-bin as $\textbf{c}   \in \mathbb{C}^{1 \times f_{bins}} $ and an arbirtary input $\textbf{x} \in \mathbb{C}^{1 \times f_{bins}} $. Thus, the inner representation of the Normal hearing model, for a given input signal $x$, is given by the matrix product, $\textbf{N} \textrm{diag}(\textbf{x})$, where $\textrm{diag}(\textbf{x})$ is the diagonal matrix with $\textbf{x}$ in the diagonal, and the inner representation of a hearing impaired model for the compensated signal, is given by the matrix product $\textbf{D} \textrm{diag}(\textbf{c}) \textrm{diag}(\textbf{x})$.

Then, an optimal compensation strategy can be found by solving the following optimization problem:
\begin{equation}
    \displaystyle{\min_{\textbf{c}}} ||\textbf{N} \textrm{diag}(\textbf{x})-\textbf{D} \textrm{diag}(\textbf{c})\textrm{diag}(\textbf{x})||_F^2
\end{equation}
Importantly, this is equivalent to finding an optimal time-domain filter, to compensate for the MSE between the time-representation between the two auditory models.

Denoting the asteriks superscript as the hermitian transpose $(^*)$ it is straightforward to show that the optimal solution is given by:
\begin{equation}
    \textbf{c} = (\textbf{H}^* \textbf{H} \odot \textbf{I})^{-1}  (\textbf{H}^* \textbf{N} \odot \textbf{I}) \textbf{1}
\end{equation}

Here, the inner product is a product across filters with different CF's at a fixed frequency bin(i), implying that an optimal gain at each frequency bin can be found by considering a weighted combination of all auditory filters at the given CF. To see this, consider a simple case where the auditory model is given by the gammatone filter: $n(f,cf,b,n) = (1+j(f-cf)b^{-1})^{(-n)} + (1+j(f+cf)b^{-1})^{(-n)}$ and $g(n) = \alpha_{cf} n(f,cf,b,n)$  . If the bandwidth is constant for all frequencies, the function is conjugate-symmetric in the first two arguments, i.e. $n(f,cf,b,n) = n(cf,f,b,n)^*$
In such a case Equation \ref{eq:optimal_c_i} collapses to:
\begin{align*}
    c_i &= \sum_{cf}\dfrac{\alpha_{cf} g(f,cf,b,n)^* g(f,cf,b,n)}{\alpha_{cf}^2 g(f,cf,b,n)^* g(f,cf,b,n)}  | _{f = i} \\ &= \sum_{f}\dfrac{\alpha_{cf} |g(cf,f,b,n)|^2}{\alpha_{f}^2 |g(cf,f,b,n))|^2} | _{f = i}
\end{align*}
The equations above imply that the ability to reconstruct a signal will be determined by a relation between the shape of the auditory filters, in particular the dB/octave of the stop-band, and the slope of the hearing loss, not the magnitude of the hearing loss.
The squared slope of the filter can be found by:
\begin{equation}
    
\end{equation}

For all these experiments, we will consider a a  1st order gammatone filterbank, using 128 log-spaced CFS between 100 Hz. and 10000 Hz, with the Q-factor linearly increasing from 0 at 100 Hz to 10 at 10 kHz. The hearing loss is simulated by a scalar loss at each CF, corresponding to the hearing loss. The increased bandwidth of the hearing-impaired critical filters are simulated by the following equation at each CF: \begin{equation}
    Q_{HI} = max((Q_{NH}-Q_{NH} \dfrac{HL}{HL_{max}}+1,1)
\end{equation}

\subsection{Number of CFs}
In order to make the training and the size of the auditory model emulator less computationally demanding, we would like to know how many CFs are needed, and how they should be spaced, in order for the auditory model to be representative of the auditory pathway. We do this, by constructing the a linear problem:
There are two linear auditory models, one describing normal hearing and another describing impaired hearing, and we wish to find a linear compensation strategy, that minimizes the difference between the impulse response of the normal hearing auditory model and the impaired hearing auditory model. Importantly, the time-frequency channels of the auditory model with impaired hearing will tend to have wider tuning and lower gain, as compared to the auditory model of normal hearing.

Mathematically, We construct the problem as follows:
For each auditory model, we generate a toeplitz matrix from the impulse response of the auditory model at each characteristic frequency (CF). We stack all these toeplitz matrices, and we denote the resulting stacked matrices as $\textbf{N}$ and $\textbf{D}$, denoting normal and impaired hearing respectively. The stacked matrices have dimensions ($(t\cdot k) \times t$), where k is the number of CFs and t is the length of the impulse response. Additonally, we define a compensation matrix $\textbf{C}$ and a speech signal \textbf{x} of dimension $(t \times 1)$.

In order to find C, we can formulate the optimization problem stated in the preceding paragraphs as:
\begin{equation}
    \displaystyle{\min_{\textbf{C}\in \textbf{R}^{t \times t}}} ||\textbf{N} \textbf{x}-\textbf{D}\textbf{C} \textbf{x}||^2 = \displaystyle{\min_{\textbf{C}\in \textbf{R}^{t \times t}}} (\textbf{N} \textbf{x}-\textbf{D}\textbf{C} \textbf{x})^T(\textbf{N} \textbf{x}-\textbf{D}\textbf{C} \textbf{x}).
\end{equation} 

\begin{comment}
this optimization problem is convex in \textbf{C}, since \begin{equation}\dfrac{\partial||\textbf{N} \textbf{x}-\textbf{D}\textbf{C} \textbf{x}||^2}{\partial^2 \textbf{C}} = \textbf{D}^T\textbf{D} \textbf{x} \textbf{x}^T \end{equation}, e.g a product of two positive semi-definite matrices. \hfill
\linebreak
\end{comment}

A minimal-norm solution can be found using the following:
\begin{equation}
    \dfrac{\partial||\textbf{N} \textbf{x}-\textbf{D}\textbf{C} \textbf{x}||^2}{\partial \textbf{C}} = 2 \textbf{D}^T \textbf{D} \textbf{C} \textbf{x} \textbf{x}^T - 2 \textbf{D}^T \textbf{N} \textbf{x} \textbf{x}^T,
\end{equation}
and equating to the zero-matrix gives:
\begin{equation}
    2 \textbf{D}^T \textbf{D} \textbf{C} \textbf{x} \textbf{x}^T - 2 \textbf{D}^T \textbf{N} \textbf{x} \textbf{x}^T = 0 \iff \textbf{C} = (\textbf{D}^T \textbf{D})^{-1} \textbf{D}^T \textbf{N} = \textbf{D}^{\dagger} \textbf{N}.
\end{equation}

Using C, we can plot the compensation strategy for different CF-spacing configurations. For this, particular work, we use the inner-hair-cell output, as this is where the frequency decomposition takes place in the auditory model. Too few CFs will cause the auditory filters to have a large amount of non-overlap in the stop-bands. This non-overlap, will cause a "ringing"-like behaviour in the final compensation strategy,  since the loss function is computed over all the CF's, and the loss function will punish any error in the gaps between CFs to a much lower degree, than in the pass-bands, allowing the  compensation strategy to freely optimize the response in the pass-band of the auditory filters, at the expense of the performance of the stop-bands in between the filters.
